# Supplementary material for: SpaBERT: A Pretrained Language Model from Geographic Data for Geo-Entity Representation
Source: arXiv:2210.12213 source file (2022-10-21)
Supplement: Supplementary file 1 [file 5_appendix.tex]

\newpage
\appendix

% The historical map is not geo-referenced. Thus geo-entity locations are in the image coordinates. 

\section{Annotation Details for the USGS to Wikidata Linking Dataset}\label{sec:appendix_annotation}
We hired three undergraduate students (not the co-authors) to transcribe text labels on the USGS maps. They drew bounding boxes/polygons around text labels and transcribed the text string to indicate geo-entity names and their locations. The results were verified and corrected by another undergraduate student and one Ph.D. student. Then, we ran an automatic script to find the potential corresponding geo-entity in Wikidata by matching their names. The collected Wikidata URIs were noisy, and we had one Ph.D. student verify the URIs by marking them as True or False linking. The verification results are randomly further reviewed by a senior digital humanities scholar specialized in the representation and reception of historical places.
